# Supplementary material for: Minimal Pole Representation and Controlled Analytic Continuation of Matsubara Response Functions
Source: arXiv:2312.10576 ancillary file (2024-06-12)
Supplement: Supplementary file 1 [file supplement.pdf]

# Supplemental Material for "Minimal Pole Representation and Controlled Analytic Continuation of Matsubara Response Functions"

Lei Zhang[1] and Emanuel Gull[1]

[1]*Department of Physics, University of Michigan, Ann Arbor, Michigan 48109, United States of America*

(Dated: June 12, 2024)

## I. DETAILS OF NUMERICAL SIMULATIONS

The input of our simulations is an odd number of Matsubara points $G(i\omega_n)$ sampled on a uniform grid

$$\{i\omega_{n_0}, i\omega_{n_0+\Delta n}, \cdots, i\omega_{n_0+(N_\omega-1)\Delta n}\}, \tag{1}$$

where $\omega_n = \frac{(2n+1)\pi}{\beta}$ for fermions and $\frac{2n\pi}{\beta}$ for bosons, $n_0 \geq 0$ is an integer controlling the number of the first few points we decide to discard (if any), $\Delta n \geq 1$ is an integer controlling the distance of successive sampling points, $N_\omega$ is the total number of sampling points and should be an odd number. We find that it is sometimes advantageous to choose $n_0$ different from 0 (for fermions) or 1 (for bosons). In this case, the final interpolant has to be validated at the discarded points to ensure that they are consistent with the interpolant.

To achieve best performance, we choose the following heuristic criteria: $n_0$ should be chosen as the smallest value so that $\min |i\omega_{n_0} - \xi_l|$ and $\max |i\omega_{n_0} - \xi_l|$ are of the same order and function values between first two sampling points, i.e., $G(i\omega_{n_0})$ and $G(i\omega_{n_0+\Delta n})$, do not change dramatically; $N_\omega$ should be chosen to the value making $\{\tilde{\xi}_l\}$ separated as far as possible; it is sufficient to set $\Delta n = \max\{1, \frac{\beta}{200}\}$ for the 64-bit machine precision. Spectra should be robust to whatever choice of $\Delta n$ and $N_\omega$ is taken. For concreteness, in our simulations we choose $\beta = 200$, $N_\omega = 2001$ and $\Delta n = 1$ for all cases; other choices show similar results.

For this paper, unless specified, the Matsubara data is always obtained from a known spectral function $A(\omega)$ via

$$G(i\omega_n) = \int_{-\infty}^{+\infty} d\omega \frac{A(\omega)}{i\omega_n - \omega} \ . \tag{2}$$

After obtaining pole information by our method, the recovered spectral function is obtained from

$$A_{\text{cont}}(\omega) = -\frac{1}{\pi} \text{Im} \lim_{\eta \to 0^+} \sum_{l=1}^{M} \frac{A_l}{\omega + i\eta - \xi_l} \ . \tag{3}$$

And the quality of the analytic continuation is characterized by the $\ell^1$ norm of the discrepancy:

$$err(A) = \int_{-\infty}^{+\infty} d\omega |A(\omega) - A_{\text{cont}}(\omega)| \ . \tag{4}$$

For broadened peaks, since poles are away from the real axis, we take $\eta \equiv 0$. For delta peaks, $\eta$ is always chosen to be 0.01 for both visualization and evaluation of $err(A)$, unless otherwise specified.

To facilitate later discussions, two functions, the Gaussian function and the Lorentzian function, are defined here:

$$g(\omega, \mu, \sigma) = \frac{1}{\sqrt{2\pi}\sigma} \exp\left\{-\frac{(x-\mu)^2}{2\sigma^2}\right\} \ , \tag{5}$$

$$l(\omega, \mu, \gamma) = \frac{1}{\pi} \frac{\gamma}{(\omega-\mu)^2 + \gamma^2} \ . \tag{6}$$

### A. FIG 2

For fig 2, we simulate two models, one for the discrete case with both centered and off-centered delta peaks, the other for the continuous case with multiple-featured broadened peaks. For the former, the spectral function takes the form:

$$A(\omega) = 0.52\delta(\omega) + 0.48\delta(\omega - 1) \ , \tag{7}$$

| $\varepsilon$ | $M$ | $A_l$ | $\xi_l$ |
|---|---|---|---|
| $2.55 \times 10^{-4}$ | 2 | 0.511333354898343 | −0.005233280979342 |
| | | 0.489020327225432 | 0.995141438211015 |
| $7.98 \times 10^{-6}$ | 2 | 0.519686962815029 | −0.000294257935939 |
| | | 0.480312064764053 | 1.000123355664247 |
| $1.83 \times 10^{-7}$ | 2 | 0.519996253000921 | −0.000005670340152 |
| | | 0.480003446182263 | 1.000008012212157 |
| $5.75 \times 10^{-9}$ | 2 | 0.520000036501130 | −0.000000005157088 |
| | | 0.479999958687507 | 1.000000183105766 |
| $1.60 \times 10^{-10}$ | 2 | 0.520000015775204 | 0.000000013352668 |
| | | 0.479999984193619 | 0.999999995909646 |
| $8.26 \times 10^{-13}$ | 2 | 0.520000000194287 | 0.000000000223985 |
| | | 0.479999999801583 | 0.999999999848198 |

TABLE I. Recovered results for fig 2(a).

where $\delta(w)$ is the Dirac delta function and the parameter $n_0$ is chosen to be 30 because of the singularity on the origin. For the later, we choose

$$A(\omega) = 0.2g(\omega, -2, 0.5) + 0.3g(\omega, 0, 0.2) + 0.5g(\omega, 1, 0.5) \tag{8}$$

with parameter $n_0 = 0$.

Recovered results are listed in Table I and II, where the negligible imaginary part for the discrete case has been discarded for readability. Distinguishing delta peaks and broadened peaks can be easily achieved by examining the imaginary part of $\xi_l$. Poles with negligible weights have also been discarded. Besides, there is subtlety associated with the predetermined error tolerance $\varepsilon$. When $\varepsilon$ is given, the program looks for the first singular value from SVD which satisfies $\sigma \leq \varepsilon$. Because we do not distinguish $\varepsilon$ and $\sigma$ in the content of our paper and $\sigma$ is discrete, $\varepsilon$ is also discrete in this sense. This is the reason why $\varepsilon$ has several digits.

### B. FIG 3

In this part, we examine density of states in $2d$ tight-binding models, as well as a ‘Kondo’-like spectral function with both smooth and sharp features.

In (a), we study the model on the square lattice with nearest-neighbor interaction $t = 1$ and next-nearest-neighbor interaction $t' = 0.2$. Following the convention from Ref. [1], the spectral function can be expressed as

$$A(\omega) = \frac{1}{\pi^2 |t'| \sqrt{z_0(u^2-4)}} K\left(\frac{z_1}{z_0}\right) , \tag{9}$$

where $K(m) = \int_0^{\frac{\pi}{2}} d\phi [1 - m \sin^2\phi]^{-1/2}$ is the complete elliptic integral of the first kind, and

$$z_0 = \begin{cases} q, & 0 < p \leq q \\ p, & 0 < q < p \\ p - q, & q < 0 \end{cases} , \tag{10}$$

$$z_1 = \begin{cases} q - p, & 0 < p \leq q \\ p - q, & 0 < q < p \\ p, & q < 0 \end{cases} . \tag{11}$$

Here, $p$ and $q$ are defined by two dimensionless parameters $u = t/t'$ and $E = \omega/t$:

$$p = \frac{4u(u-E)}{u^2-4} , \tag{12}$$

$$q = \frac{(Eu-4)^2}{4(u^2-4)} . \tag{13}$$

| $\varepsilon$ | $M$ | $A_l$ | $\xi_l$ |
|---|---|---|---|
| $2.36\times10^{-3}$ | 3 | $0.118058903808435+0.182403162681001i$ | $-1.204450173782112-0.156711479499872i$ |
| | | $0.623126378429802-0.167121980005347i$ | $-0.030090705376894-0.293343960793297i$ |
| | | $0.315285665426528-0.002154502881458i$ | $1.048877531307533-0.111010313119802i$ |
| $1.89\times10^{-5}$ | 4 | $0.294789142930615-0.030683407576160i$ | $-1.946519611154891-0.483902193898281i$ |
| | | $0.195404650709736-0.620495075034599i$ | $-0.146585427014933-0.335878950110814i$ |
| | | $-0.029769767413130+0.374041799008952i$ | $0.177981280484458-0.295491343144327i$ |
| | | $0.534054140868870+0.274005525859195i$ | $1.206305940667271-0.475472509411325i$ |
| $7.70\times10^{-7}$ | 5 | $0.235930048552452-0.078646824324015i$ | $-2.136509145947329-0.415697321174864i$ |
| | | $-0.246758054089975-0.960556415150371i$ | $-0.174493698730584-0.399719372355751i$ |
| | | $0.137210004779730+1.154077808958321i$ | $0.138510559424034-0.403564765336938i$ |
| | | $0.958566688287725-0.395613126648794i$ | $0.786369292495720-0.692579926695643i$ |
| | | $-0.085315624707392+0.281372452486608i$ | $1.734960150099575-0.630973836857521i$ |
| $1.04\times10^{-9}$ | 8 | $-0.000869254038466-0.066370182984203i$ | $-2.784179904883692-0.471055373757732i$ |
| | | $0.251842355381606-0.000121368742237i$ | $-1.943630489721618-0.571923148208484i$ |
| | | $-0.173694882612084-0.087756520613306i$ | $-0.806323900759767-0.637092057687596i$ |
| | | $-1.852955505830634+0.578497739787043i$ | $-0.262523270780438-0.514116078156992i$ |
| | | $4.632053629971353-0.456112255262277i$ | $-0.006147361455948-0.525774338640829i$ |
| | | $-2.337119090834560-0.482155607092420i$ | $0.253151690147532-0.523458691783798i$ |
| | | $0.601579319546361+0.449531659601334i$ | $1.204948811727744-0.733105192605620i$ |
| | | $-0.120836019433872+0.064484991851313i$ | $1.946971017902517-0.674348076546615i$ |
| $3.54\times10^{-11}$ | 9 | $-0.035616516363429-0.085123955396923i$ | $-2.771552714415409-0.603953536741066i$ |
| | | $0.347803557080295+0.027535918871576i$ | $-1.928181641845855-0.700395552874667i$ |
| | | $-0.799529779639230+0.045638491582258i$ | $-0.640111461899102-0.956402202375529i$ |
| | | $-1.544146981258659+1.760650223719916i$ | $-0.292521122921537-0.540703723620048i$ |
| | | $5.654018960196657-2.147975691168267i$ | $-0.027662643155237-0.544480942308326i$ |
| | | $-3.050137945302188-0.175769757941538i$ | $0.234638870973690-0.533138493156489i$ |
| | | $-0.000037772920485+0.000069877726134i$ | $0.548923094314165-0.031530914939886i$ |
| | | $0.539369205783499+0.546534384372247i$ | $1.254717651072944-0.746514675519833i$ |
| | | $-0.111722512793357+0.028440919741972i$ | $2.007471710919555-0.696705820338941i$ |
| $2.14\times10^{-13}$ | 11 | $-0.024837926566027-0.004366347509901i$ | $-3.118069119689864-0.643167785434883i$ |
| | | $0.098395494318060-0.219620264536520i$ | $-2.365185683165514-0.716876112030249i$ |
| | | $0.185967844930931+0.252384802247341i$ | $-1.674049451686480-0.785786582368154i$ |
| | | $0.924104691602651+0.664403394148004i$ | $-0.397811568145370-0.560220818702668i$ |
| | | $-4.265344958424443-4.603656276549160i$ | $-0.157425734776960-0.577214844399315i$ |
| | | $5.440160882854892+6.435022023450554i$ | $0.059136250873121-0.581043116187629i$ |
| | | $-1.677223757359942-2.886437519921194i$ | $0.288553682833324-0.574535166568495i$ |
| | | $0.034681571989394-0.069689910633521i$ | $0.814058514940610-0.481768187664549i$ |
| | | $0.346643348885711+0.325386507633010i$ | $1.261498342766544-0.664043673218963i$ |
| | | $-0.050313356223844+0.105058861667653i$ | $1.793090553825032-0.586679051877780i$ |
| | | $-0.012233839679708+0.001514730029528i$ | $2.364554990881565-0.552750542706448i$ |

TABLE II. Recovered results for fig 2(b).

And finally, the non-zero range is determined by

$$-4-\frac{4}{u}\le E\le 4-\frac{4}{u},\qquad |u|\ge 2. \tag{14}$$

Because of the sharp feature in the spectral function, we find that calculating Matsubara data from Eq. 2 loses lots of precision. So instead, we obtain the input data from

$$G(i\omega_n)=\frac{1}{(2\pi)^2}\int_{-\pi}^{\pi}dk_1\int_{-\pi}^{\pi}dk_2\frac{1}{i\omega_n-\epsilon_k}\ , \tag{15}$$

where the tight-binding Hamiltonian has the expression

$$\epsilon_k = -2t\cos k_1 - 2t\cos k_2 - 4t'\cos k_1 \cos k_2 \ . \tag{16}$$

The simulation is performed at $n_0 = 0$.

In (b), we study the model on the Bethe lattice with interaction $t = 1$. The spectral function in this case is a semicircle:

$$A(\omega) = \frac{1}{2\pi t^2}\sqrt{4t^2 - \omega^2} \ . \tag{17}$$

And the Matsubara Green's function has the analytic expression

$$G(i\omega_n) = \frac{i}{2t^2}(\omega_n - \sqrt{\omega_n^2 + 4t^2}) \text{ for } \omega_n > 0 \ . \tag{18}$$

This is also simulated at $n_0 = 0$.

In (c), we study the model on an anisotropic triangular lattice with interaction $t = 1$ for two of the three directions and $t' = 0.75$ for the third direction. As shown in Ref. [1], the spectral function has the analytic form

$$A(\omega) = \frac{1}{\pi^2 t'\sqrt{z_0}} K\left(\frac{z_1}{z_0}\right) \ , \tag{19}$$

where

$$z_0 = \begin{cases} q, & 0 < \ p \leq q \\ p, & 0 < \ q < p \\ p - q, & \quad q < 0 \end{cases} \ , \tag{20}$$

.

$$z_1 = \begin{cases} q - p, & 0 < \ p \leq q \\ p - q, & 0 < \ q < p \\ p, & \quad q < 0 \end{cases} \ . \tag{21}$$

After the definition of two dimensionless parameters $u = t/t'$ and $E = \omega/t$, $p$ and $q$ can be expressed as

$$r = u\sqrt{u^2 - Eu + 2} \ , \tag{22}$$

$$p = 4r \ , \tag{23}$$

$$q = \frac{(r - u^2)^2(r^2 - 4u^2 + 2ru^2 + u^4)}{4u^4} \ . \tag{24}$$

The non-zero range is

$$-4 - \frac{2}{u} \leq E \leq u + \frac{2}{u}, \qquad 0 < u \leq 2 \ , \tag{25}$$

$$-4 - \frac{2}{u} \leq E \leq 4 - \frac{2}{u}, \qquad u > 2 \ . \tag{26}$$

Similarly, we find the Matsubara data calculated from Eq. 2 is also inaccurate. So instead, we obtain the input data from Eq. 15 with the Hamiltonian

$$\epsilon_k = -2t\cos k_1 - 2t'\cos k_2 - 2t\cos(k_1 - k_2) \ . \tag{27}$$

Simulation is performed at $n_0 = 0$.

Finally, the spectral function in (d) has the form

$$A(\omega) = 0.2g(\omega, -2, 0.5) + 0.6\delta(\omega) + 0.2g(\omega, 2, 0.5) \ , \tag{28}$$

with $n_0 = 10$ is chosen for the simulation. For the inset, $\eta$ is chosen to be a different value 0.001 to give a better visualization of the comparison.

Simulations for Maximum Entropy (MaxEnt) method and stochastic optimization method (SOM) are performed using the programs in Refs. [2] and [3], respectively. The parameter $\sigma_n$ for MaxEnt is fine-tuned to yield the best possible spectrum, with values set at $10^{-5}$, $10^{-4}$, $10^{-5}$ and $10^{-3}$, respectively. The weight factor $S(n)$ is set to be 1 for SOM.

### C. FIG 4

In (a) and (b), we perform simulations on fermionic grids and choose $n_0 = 0$ for both cases. For the former, the spectral function reads

$$A(\omega) = -0.5g(\omega, -3, 0.5) + 0.1g(\omega, -1, 1) - 0.1g(\omega, 1, 1) + 0.5g(\omega, 3, 0.5) \ . \tag{29}$$

And for the later, the spectral function is

$$A(\omega) = \sum_l A_l \delta(\omega - \xi_l) \tag{30}$$

with

$$A_l = \{-0.06842167, 0.30803739, 0.09215373, -0.28216683, -0.09213708, 0.04253446\} \ , \tag{31}$$

$$\xi_l = \{-4.63614978, -2.60745562, 0.86189661, 1.61810008, 3.33810339, 4.02550532\} \ , \tag{32}$$

which comes from the Exact Diagonalization result of a Hubbard dimer system.

For (c) and (d), simulations are performed on bosonic grids with $n_0 = 0$ and 10, respectively. The spectral function of (c) is

$$A(\omega) = -0.5g(\omega, -1, 1) + 0.5g(\omega, 1, 1) \tag{33}$$

and of (d) is

$$A(\omega) = \sum_l A_l \delta(\omega - \xi_l) \tag{34}$$

with

$$A_l = \{-0.1, -0.3, 0.2, 0.4, -0.4, -0.2, 0.3, 0.1\} \ , \tag{35}$$

$$\xi_l = \{-3, -2, -1, -0.02, 0.02, 1, 2, 3\} \ . \tag{36}$$

### D. FIG 5

We test the noise resistance of our method for both discrete and continuous cases. The discrete case is simulated at $n_0 = 0$ for

$$A(\omega) = 0.6\delta(\omega + 1) + 0.4\delta(\omega - 1) \ , \tag{37}$$

and the continuous case is simulated at $n_0 = 10$ for

$$A(\omega) = 0.3l(\omega, -2.5, 0.8) + 0.5l(\omega, 0, 0.5) + 0.2g(\omega, 2.5, 0.8) \ . \tag{38}$$

Noise is added to the clean data by

$$G_{\text{noisy}}(i\omega_n) = G_{\text{exact}}(i\omega_n)(1 + \delta \times N_{\mathbb{C}}(0, 1)) \ , \tag{39}$$

where $\delta \in \{10^{-6}, 10^{-5}, 10^{-4}, 10^{-3}, 10^{-2}\}$ and $N_{\mathbb{C}}(0, 1)$ is the complex-valued normal Gaussian distribution. The input data we used is also included in the folder.

The parameter $\sigma_n$ for performing MaxEnt is set to be $0.01 \times |G_{\text{noisy}}(i\omega_n)|$. We do not use $\sigma_n = \delta \times |G_{\text{noisy}}(i\omega_n)|$ for MaxEnt because it will cause the sawtooth noise instability. The weight factor $S(n)$ for SOM is also set to be proportional to $|G_{\text{noisy}}(i\omega_n)|$.

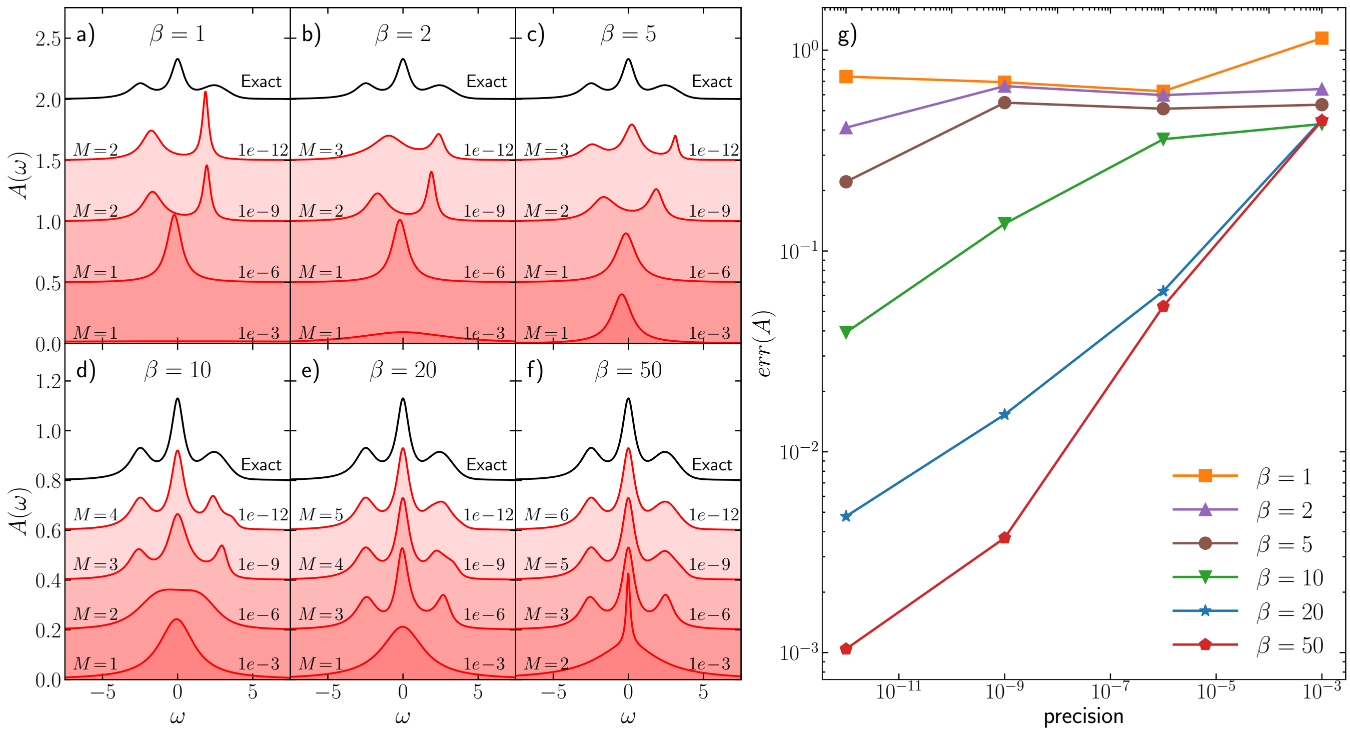


FIG. 1. Recovered spectral functions at different temperatures $\beta \in \{1, 2, 5, 10, 20, 50\}$ and various precision levels $\{10^{-3}, 10^{-6}, 10^{-9}, 10^{-12}\}$. Left panel: evolution of spectrum shapes. Right panel: convergence of $err(A)$ as a function of precision. Number of available data points is fixed at $N_\omega = 201$.

## II. DEPENDENCE ON TEMPERATURE

To explore the dependence of performance on system temperature, we take the model 38 as an example and perform simulations over a wide range of temperatures and various levels of precision. Explicitly, data points at precision $10^{-m}$ are obtained by

$$G_{\text{prec}}(i\omega_n) = \text{round}(G_{\text{exact}}(i\omega_n) \times 10^m) \times 10^{-m} \ . \tag{40}$$

As shown in Fig. 1, the results improve as precision increases, regardless of the temperature. However, as temperature increases, the convergence rate becomes slower and thus higher precision is needed to resolve the same feature, which is an inherent difficulty of the analytic continuation problem.

Although the three-peak feature cannot be resolved at the current precision for $\beta = 1$ and 2, we argue that there is still an improvement in the results. To illustrate this, we calculate the difference between the exact spectrum moments $A_k$ and the recovered ones $\hat{A}_k$. These are calculated using the following equations:

$$A_k = \int_{-\infty}^{\infty} d\omega A_{\text{exact}}(\omega)\omega^k \quad \text{and} \quad \hat{A}_k = \sum_l A_l \xi_l^k \ . \tag{41}$$

As shown in Fig. 2, the recovered moments become more and more accurate when the precision increases. It is expected that as the precision is improved further, different peaks can eventually be resolved.

## III. DEPENDENCE ON AVAILABLE DATA POINTS

To explore the dependence on available data points, we fix the system at a moderate temperature ($\beta = 30$) and perform simulations for model 38 with a varying number of data points $N_\omega \in \{7, 9, 11, 35, 151, 1001\}$. As shown in Fig. 3, while seven points are not enough to achieve convergence, nine points are sufficient to resolve the three-peak feature. For $N_\omega \geq 11$, we observe a similar convergence behavior, which is insensitive to the number of available

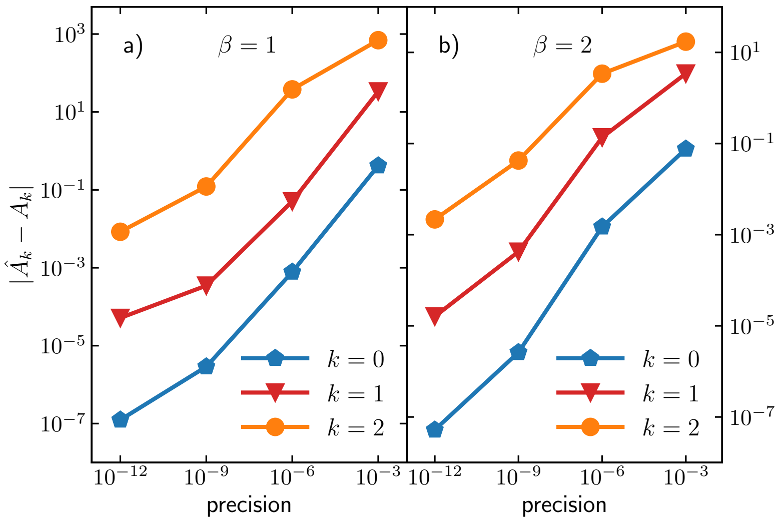


FIG. 2. Convergence of spectrum moments as a function of precision for $\beta = 1$ and 2.

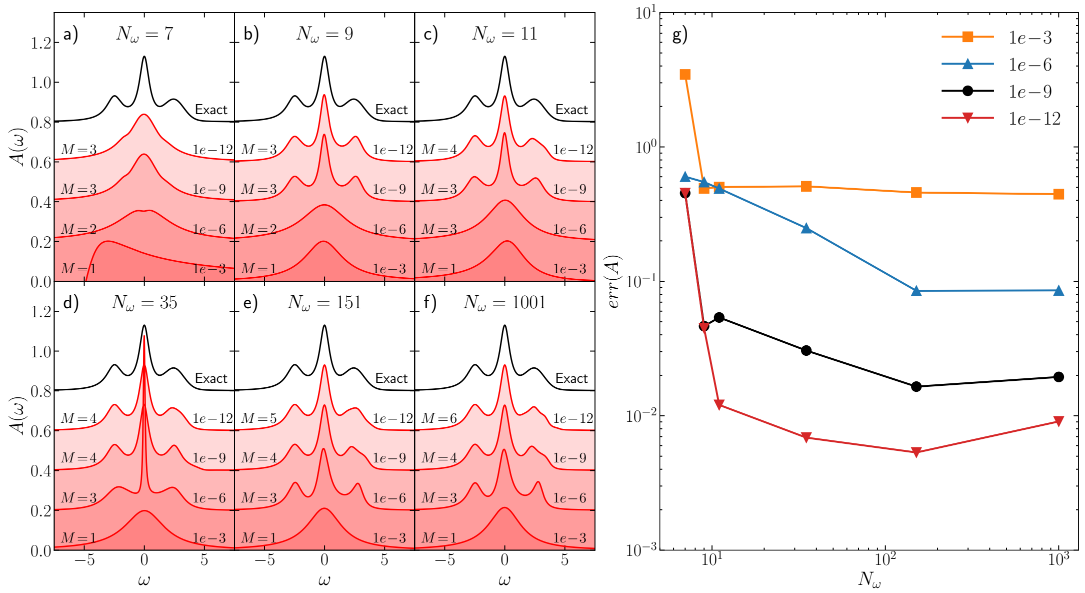


FIG. 3. Recovered spectral functions at different numbers of data points $N_\omega \in \{7, 9, 11, 35, 151, 1001\}$ and various precision levels $\{10^{-3}, 10^{-6}, 10^{-9}, 10^{-12}\}$. Left panel: evolution of spectrum shapes. Right panel: convergence of $err(A)$ as a function of $N_\omega$ at different precision levels. System temperature is fixed at $\beta = 30$.

points. Specifically, increasing the number of data points does not necessarily accelerate convergence. We note that the reason for this phenomenon is due to the fact that the holomorphic mapping eliminates the effects from the absence of data points in the long tail. This happens because the information of mapped poles is fully contained by function values on the unit circle, which are only mapped from the finite interval $[i\omega_{n_0}, i\omega_{n_0+(N_\omega-1)\Delta n}]$. When there are too many data points, the convergence speed slightly slows down, as the mapped poles become too close to each other. Given $N_\omega = 2N + 1$ data points, our method can recover at most $N$ poles, leading to failures when there are too few points to capture all poles. We estimate the threshold for the required number of points to be $N_{\rm min} \gtrsim 2N_{\rm pole} + 1$, where $N_{\rm pole}$ is the number of poles needed to resolve the fine structure of the spectrum. When $N_\omega \geq N_{\rm min}$, convergence should always be observed at sufficient precision.

[1] Y. Yu, S. Li, S. Iskakov, and E. Gull, Phys. Rev. B **107**, 075106 (2023).

[2] R. Levy, J. LeBlanc, and E. Gull, Computer Physics Communications **215**, 149 (2017).

[3] I. Krivenko and M. Harland, Computer Physics Communications **239**, 166 (2019).
